# Supplementary material for: Nanoscale Dipolar Fields in Artificial Spin Ice Probed by Scanning NV Magnetometry
Source: arXiv:2509.02233 ancillary file (2026-09-21)
Supplement: Supplementary file 1 [file supplement.pdf]

## Supplementary Material

### Nanoscale Dipolar Fields in Artificial Spin Ice Probed by Scanning NV Magnetometry

Ephraim Spindler,<sup>1,\*</sup> Vinayak Shantaram Bhat,<sup>2</sup> Elke Neu,<sup>1</sup> Mathias Weiler,<sup>1</sup> and M. Benjamin Jungfleisch<sup>2</sup>

<sup>1</sup>*Fachbereich Physik and Landesforschungszentrum OPTIMAS, Rheinland-Pfälzische Technische Universität Kaiserslautern-Landau (RPTU), 67663 Kaiserslautern, Germany*

<sup>2</sup>*Department of Physics & Astronomy, University of Delaware, Newark, DE 19716, USA*

#### S1. SAMPLE FABRICATION

A bilayer electron beam resist, consisting of a copolymer and polymethyl methacrylate, is spin-coated onto a high-resistance silicon substrate. The resist is subsequently baked at 170 °C for two minutes to enhance adhesion and stability. Artificial spin ice (ASI) arrays, arranged in a square lattice, are patterned using a 100 keV electron beam lithography system.

The exposed resist is developed in a 1:1 solution of methyl isobutyl ketone and isopropyl alcohol, followed by rinsing in isopropyl alcohol to remove residual chemicals. After development, a 25 nm-thick Ni<sub>81</sub>Fe<sub>19</sub> film with a 3 nm Al capping layer is deposited via electron beam evaporation at a base pressure of 10<sup>-6</sup> mBar. The liftoff process is performed by immersing the processed silicon wafer in an N-methyl-2-pyrrolidone solution, which effectively dissolves the resist while preserving the patterned nanostructure arrays on the substrate.

Each nanomagnet measures approximately 110 nm in width and 810 nm in length (Figure S1). The lattice constants for samples *S-A* and *S-B* are 1000 nm and 910 nm, respectively. All nanomagnets are rotated by 45° to ensure full saturation under a magnetic field applied along the x-axis.

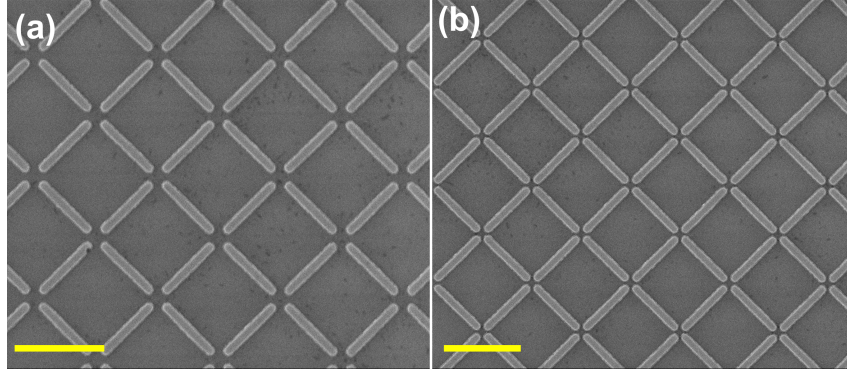

FIG. S1. Representative scanning electron microscopy (SEM) images of the ASI samples (a) *S-A* and (b) *S-B*, with yellow scale bars indicating 1  $\mu\text{m}$ .

A topography scan on sample *S-B* is performed using the atomic force microscopy platform integrated into the scanning NV microscope, utilizing a conventional silicon tip (A-Probe, Akiyama) for enhanced spatial resolution. The 2D scan is shown in the upper right corner of Fig. S2. A cross-section is extracted along line *s* (indicated in the 2D image), averaging across 40 pixels. The results indicate that the total nanomagnet height is about 26.7 nm, which is approximately 5% smaller than the expected deposition thickness. Considering a capping layer thickness of 3 nm, this corresponds to a magnetic layer thickness of approximately 23.7 nm, which is close to the 25 nm value used in the micromagnetic simulations. Furthermore, the cross-section reveals a width ratio of approximately 2:1 between the base and the top of the nanomagnets. A first approximation of the mean width (calculated as  $(70 \text{ nm} + 147 \text{ nm})/2 = 108.5 \text{ nm}$ ) shows very good agreement with the design width of 110 nm. However, it is important to note that the radius and opening angle of the scanning tip lead to an overestimation of the width, especially in the lower parts of the cross-section, making its precise estimation challenging.

\* E-Mail: [spindler@rptu.de](mailto:spindler@rptu.de)

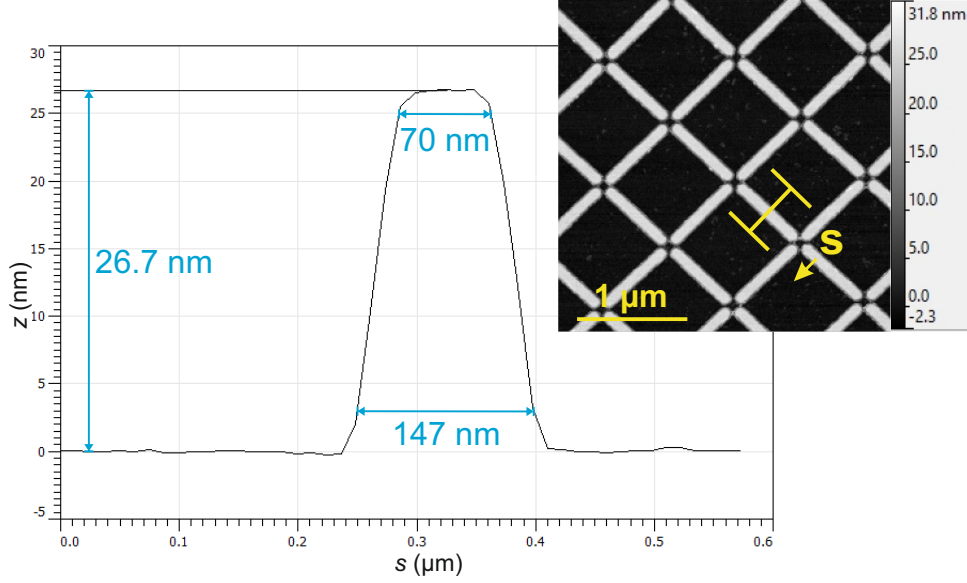

FIG. S2. Representative cross-section of one nanomagnet extracted from a topography scan on  $S$ - $B$  along the route  $s$  (height averaged across the width indicated by the bars at the beginning and end of  $s$ ) using a conventional silicon scanning tip.

## S2. DETAILS ON MICROMAGNETIC SIMULATIONS OF THE MAGNETIC GROUND STATE AND STRAY FIELD

The simulation area, centered around the vertex of interest, measures  $3\text{ }\mu\text{m} \times 3\text{ }\mu\text{m} \times 25\text{ nm}$  in  $x$ ,  $y$  and  $z$ -direction, respectively. The  $x$ - $y$  plane corresponds to the sample plane, with the  $z$ -axis perpendicular to it. It is divided into  $512 \times 512 \times 1$  cells. Each cell  $(i, j)$  has a normalized magnetization  $\mathbf{m}_{ij}$  and a magnetic moment  $\mathbf{M}_{ij} = V \cdot M_s \cdot \mathbf{m}_{ij}$ , where  $M_s = 785\text{ kA m}^{-1}$  is the saturation magnetization and  $V$  is the cell volume. We used an exchange stiffness  $A = 15\text{ pJ m}^{-1}$ . The geometry of sample  $S$ - $A$  was implemented and rotated by  $-3.6^\circ$  around the  $z$ -axis to align with the experimental setup. Before relaxing the micromagnetic system under a given external magnetic field  $\mathbf{H}_{\text{ext}}$ , an initial uniform magnetization was assigned to each nanomagnet, based on the Ising states extracted from quenching and cODMR scans presented in Fig. 2 of the main text.

The relaxed magnetization landscape is then used to calculate the dipolar stray field  $\mathbf{H}_{\text{ASI}}$  in a lifted plane at various distances from the magnetic layer surface. To do so, the individual contribution of each material cell is summed up using:

$$\mathbf{H}_{\text{ASI}}(k, l) = \sum_{i, j} \frac{1}{4\pi} \left( \frac{3\mathbf{r}_{ij \rightarrow kl} (\mathbf{r}_{ij \rightarrow kl} \cdot \mathbf{M}_{ij})}{r_{ij \rightarrow kl}^5} - \frac{\mathbf{M}_{ij}}{r_{ij \rightarrow kl}^3} \right) \quad (\text{S1})$$

where  $\mathbf{r}_{ij \rightarrow kl}$  is the vector pointing from the center of the material cell  $(i, j)$  to the position  $(k, l)$  in the lifted plane.

## S3. GRAPHICAL DESCRIPTION OF THE FULL EVALUATION ALGORITHM

The flowchart in Fig. S3 visualizes and summarizes the steps included in the modeling procedure, highlighting the stages where the final modeling results are extracted (indicated in green). The flowchart is conceptually divided into two main parts, each corresponding to distinct optimization goals. The experimentally obtained magnetic field projections  $\mu_0 H_{\parallel}$  and  $\mu_0 H_{\perp}$  are calculated from the NV center's ESR frequencies using Equations (1) and (2) of the main manuscript.

The top section of the flowchart describes the iterative process for determining the external magnetic field  $\mathbf{H}_{\text{ext}}$  and the corresponding micromagnetic state  $\mathbf{m}$ , as presented in Fig. 3 of the main text. This process begins with an initial approximation of the micromagnetic ground state  $\mathbf{m}_0$ , simulated with zero external magnetic field. Next, the ASI stray field  $\mathbf{H}_{\text{ASI}}$  is calculated in the assumed measurement plane using a first approximation of the magnetic stand-off distance in contact,  $d_{\text{MSO},0} = 75\text{ nm}$ . The obtained magnetic field data is then matched with the experimental data by multiplying  $\mathbf{H}_{\text{ASI}}$  with a factor  $c$  (to

account for the effective saturation magnetization) and vectorially adding an external field  $\mathbf{H}_{\text{ext}}$ . The resulting best-fit  $\mathbf{H}_{\text{ext}}$  is then used in a second simulation to obtain a more refined micromagnetic state ( $\mathbf{m}$ ). This updated  $\mathbf{m}$  is used for a second fitting step, which yields the final  $\mathbf{H}_{\text{ext}}$  value (highlighted in green in the flowchart).

The second part of the flowchart focuses on determining the true  $d_{\text{MSO}}$  and  $M_{\text{s,eff}}$ , which is further detailed in Fig. S4. Utilizing the refined magnetization  $\mathbf{m}$  obtained from the first part,  $\mathbf{H}_{\text{ASI}}$  is calculated for various fixed values of  $d_{\text{MSO}}$  ranging from  $d_{\text{MSO},1} = 50 \text{ nm}$  to  $d_{\text{MSO},7} = 80 \text{ nm}$ . The true  $d_{\text{MSO}}$  is identified at the point where the best agreement with the experimental data is achieved, which is also where the final  $M_{\text{s,eff}}$  is extracted.

In this final optimization step, both the scaling factor  $c$  and the external field  $\mathbf{H}_{\text{ext}}$  are included as fit parameters. The scaling factor  $c$  (which accounts for the effective saturation magnetization) is refitted for each tested value of  $d_{\text{MSO}}$ . This is crucial because the best-fit values for  $c$  and  $d_{\text{MSO}}$  are strongly correlated, and keeping  $c$  constant could artificially shift the identified minimum for  $d_{\text{MSO}}$ . This approach is analogous to the simultaneous fitting of  $d_{\text{MSO}}$  and  $M_{\text{s}}$  in analytical stray field models, which is a common method to determine the value of  $d_{\text{MSO}}$  [1–3]. The re-inclusion of  $\mathbf{H}_{\text{ext}}$  serves as a robustness check. While its value is expected to be well-constrained by the previous part, including it in this final step ensures that the determination of  $d_{\text{MSO}}$  is not biased by any potential small residual errors from the first part of the algorithm.

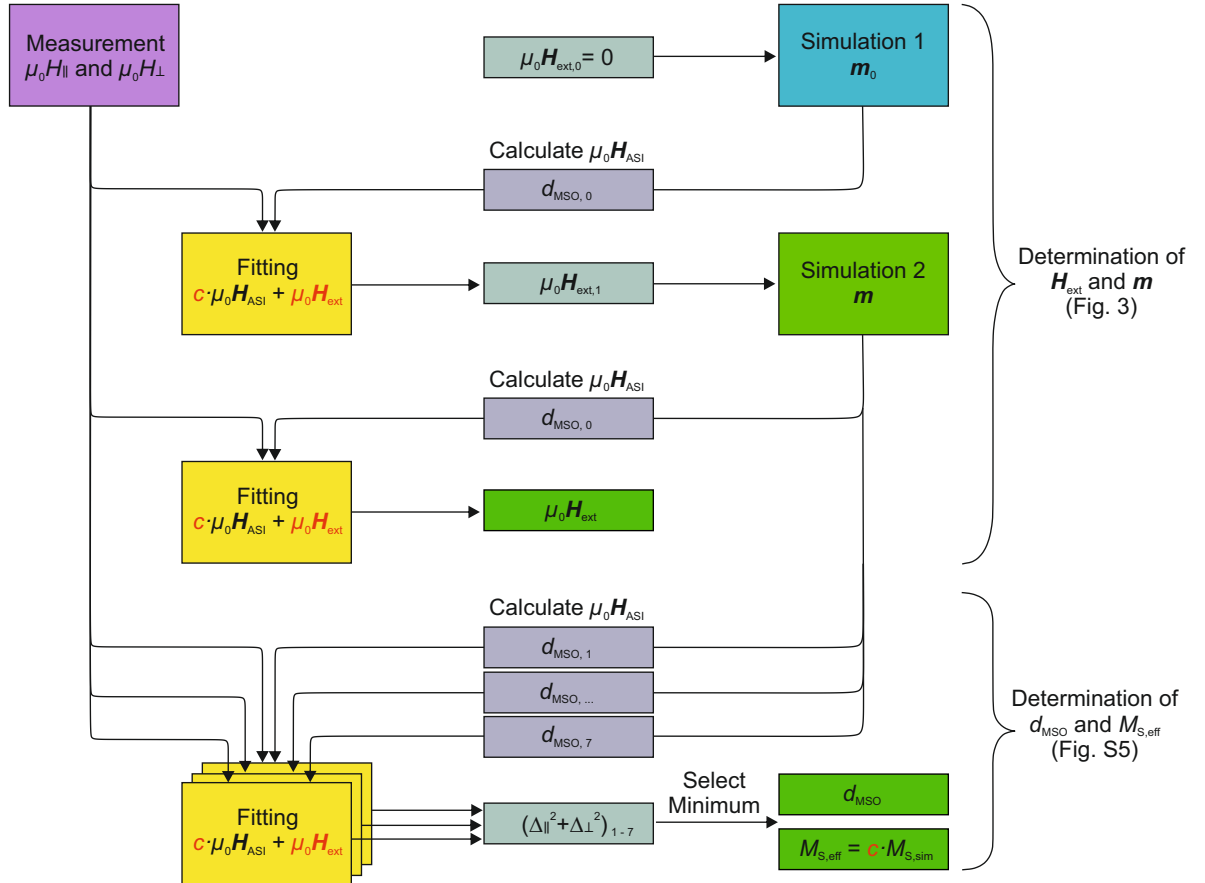

FIG. S3. Flowchart summarizing the multi-step modeling procedure used for the experimentally obtained magnetic field data. Final modeling results are highlighted in green. The diagram is conceptually divided into two parts, detailing the iterative determination of the external magnetic field ( $\mu_0 \mathbf{H}_{\text{ext}}$ ) and the corresponding micromagnetic ground state ( $\mathbf{m}$ ) (as presented in Fig. 3 of the main text), and the subsequent determination of the magnetic stand-off distance ( $d_{\text{MSO}}$ ) and effective saturation magnetization ( $M_{\text{s,eff}}$ ) (as detailed in Fig. S4).

#### S4. DETERMINATION OF SENSOR-SAMPLE DISTANCE AND EFFECTIVE SATURATION MAGNETIZATION

Following the determination of the magnetic state (as detailed in Fig. 3 of the main manuscript), the mean total error  $\Delta_{\parallel}^2 + \Delta_{\perp}^2$  is minimized by repeating the fitting of  $\mathbf{H}_{\text{ext}}$  and  $M_{\text{s,eff}}$  for different values of  $d_{\text{MSO}}$ , which are used in the calculation of the nanomagnets' stray field  $\mathbf{H}_{\text{ASI}}$ . As shown in Fig. S4, the effective saturation magnetization  $M_{\text{s,eff}} = 593 \text{ kA m}^{-1}$  is extracted at the point where this error is minimized, corresponding to  $d_{\text{MSO}} = 65 \text{ nm}$ .

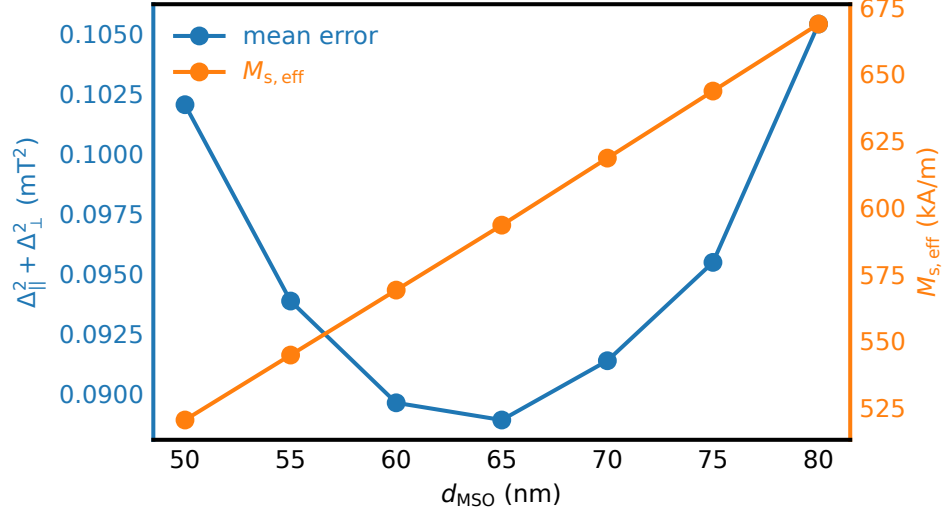

FIG. S4. Determination of  $d_{\text{MSO}}$  and  $M_{\text{s,eff}}$ . The total mean error  $\Delta_{\parallel}^2 + \Delta_{\perp}^2$  is evaluated after optimizing the external magnetic field  $\mathbf{H}_{\text{ext}}$  and the effective saturation magnetization  $M_{\text{s,eff}}$  for different values of  $d_{\text{MSO}}$ , which is used to compute the stray field  $\mathbf{H}_{\text{ASI}}$  at the measurement plane. The minimum deviation occurs at  $d_{\text{MSO}} = 65 \text{ nm}$ , corresponding to  $M_{\text{s,eff}} = 593 \text{ kA m}^{-1}$ .

#### S5. INDUCED MAGNETIZATION TILTS

The subtle tilt of the magnetization induced by an external magnetic field of  $|\mu_0 \mathbf{H}_{\text{ext}}| = 11.2 \text{ mT}$  is not readily visible in Fig. 3 of the main manuscript. Therefore, both corresponding magnetic ground states are simulated with higher resolution and presented using a more sensitive color scheme in Fig. S5(a,b). Panel (c) shows a difference image ( $\Delta \mathbf{m} = \mathbf{m}_{|\mu_0 \mathbf{H}_{\text{ext}}|=11.2 \text{ mT}} - \mathbf{m}_{|\mu_0 \mathbf{H}_{\text{ext}}|=0}$ ), demonstrating that the effect induced by the external magnetic field is most prominent at the rounded ends of the nanomagnets.

- 
- [1] J.-P. Tetienne, T. Hingant, L. Martínez, S. Rohart, A. Thiaville, L. H. Diez, K. Garcia, J.-P. Adam, J.-V. Kim, J.-F. Roch, I. Miron, G. Gaudin, L. Vila, B. Ocker, D. Ravelosona, and V. Jacques, The nature of domain walls in ultrathin ferromagnets revealed by scanning nanomagnetometry, *Nature Communications* **6**, 6733 (2015).
  - [2] N. Hedrich, D. Rohner, M. Batzer, P. Maletinsky, and B. J. Shields, Parabolic Diamond Scanning Probes for Single-Spin Magnetic Field Imaging, *Physical Review Applied* **14**, 064007 (2020).
  - [3] Z. Xu, M. L. Palm, W. Huxter, K. Herb, J. M. Abendroth, K. Bouzehouane, O. Boulle, M. S. Gabor, J. Urrestarazu Larranaga, A. Morales, J. Rhensius, G. Puebla-Hellmann, and C. L. Degen, Minimizing Sensor-Sample Distances in Scanning Nitrogen-Vacancy Magnetometry, *ACS Nano* **19**, 8255 (2025).

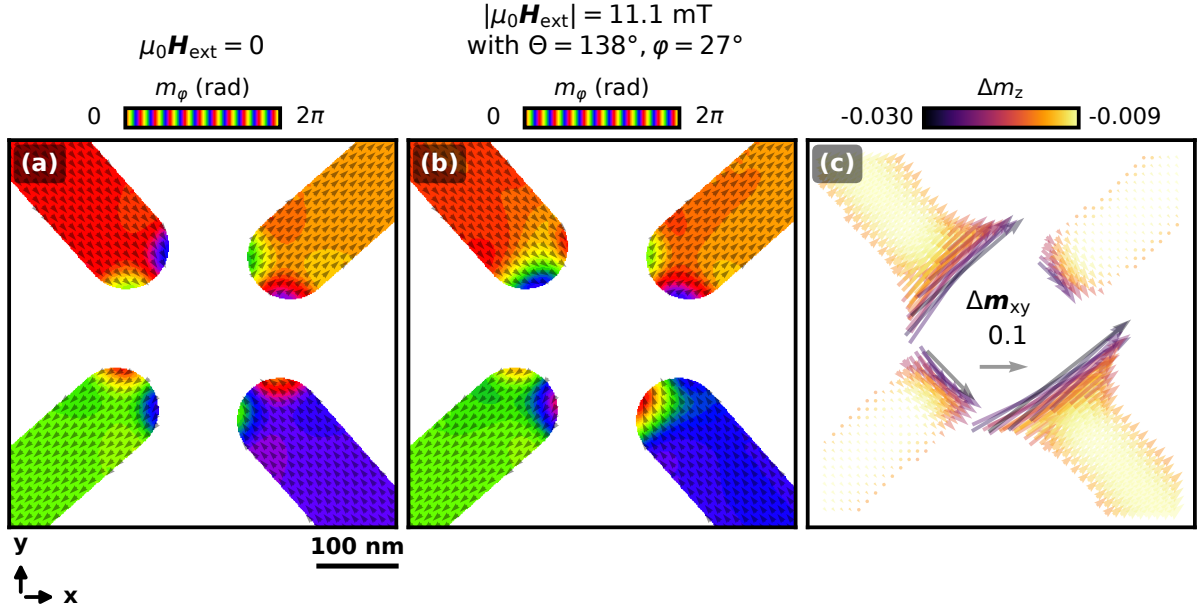

FIG. S5. (a,b) In-plane (IP) orientation of  $\mathbf{m}$  represented by the azimuthal angle  $m_\varphi$  in the vertex region of sample *S-A* (type I configuration). This visualizes the magnetization tilt at the apex of the nanomagnets (a) without an external field and (b) with an external field. The external field orientation is described using the polar and azimuthal angles  $\Theta = 138^\circ$ ,  $\varphi = 27^\circ$  corresponding to the coordinate system in the lower left corner. (c) Difference map  $\Delta \mathbf{m} = \mathbf{m}_{|\mu_0 \mathbf{H}_{\text{ext}}|=11.1 \text{ mT}} - \mathbf{m}_{|\mu_0 \mathbf{H}_{\text{ext}}|=0}$  showing the isolated effect of the magnetic field on the magnetization. The IP component  $\Delta \mathbf{m}_{xy}$  of  $\Delta \mathbf{m}$  is indicated by arrows, where the length of the arrow in the center corresponds to a value of  $|\Delta \mathbf{m}_{xy}| = 0.1$ . The out-of-plane (OOP) component  $\Delta m_z$  is encoded in the colormap.
